# Supplementary material for: Suppressed SUSY for the SU(5) Grand Unified Supergravity Theory
Source: arXiv:1706.07796 ancillary file (2017-06-26)
Supplement: Supplementary file 1 [file 5221Math.pdf]

This is a pdf of a *Mathematica* notebook deriving the results for “Suppressed SUSY for the SU(5) Grand Unified Supergravity Theory”, together with some brief explanations.

Author John Dixon, version date is June 25, 2017

In[1]:=

**DateList[]**

Out[1]= {2017, 6, 26, 7, 8, 17.2150161}

```

In[2]:= (* This is 5221Math *) (* field definitions *)
hL := {(K25 + i K30) / Sqrt[2], (K26 + i K31) / Sqrt[2],
        (K27 + i K32) / Sqrt[2], (K28 + i K33) / Sqrt[2], (K29 + i K34) / Sqrt[2]};
hR := {(K25 - i K30) / Sqrt[2], (K26 - i K31) / Sqrt[2], (K27 - i K32) / Sqrt[2],
        (K28 - i K33) / Sqrt[2], (K29 - i K34) / Sqrt[2]};
kH := {{(K3 + K8 / Sqrt[3] - 2 K12 / Sqrt[15], K1 + i K2, K4 + i K5, K13 + i K14, K19 + i K20),
        {K1 - i K2, -K3 + K8 / Sqrt[3] - 2 K12 / Sqrt[15], K6 + i K7, K15 + i K16, K21 + i K22},
        {K4 - i K5, K6 - i K7, -Sqrt[4 / 3] K8 - 2 K12 / Sqrt[15], K17 + i K18, K23 + i K24},
        {K13 - i K14, K15 - i K16, K17 - i K18, K11 + Sqrt[3 / 5] K12, K9 + i K10},
        {K19 - i K20, K21 - i K22, K23 - i K24, K9 - i K10, -K11 + Sqrt[3 / 5] K12}}};
vectorBosons := kH /. Table[Rule[Symbol["K" <> ToString[i]],
        Symbol["V" <> ToString[i]]], {i, 1, 24}];

(* apply shifts for VEVs *)
shiftAll := {K11 → K11 + MK1, K12 → K12 + MK2, K29 → K29 + MK9};
replaceAllFieldsWithZero := Table[Rule[Symbol["K" <> ToString[i]], 0], {i, 1, 34}];
replaceAllFieldsWithZero;

(* invariant quantities *)
invarH2 := Expand[hL.hR];
invarK2 := Expand[(1 / 4) Tr[kH.kH]];
kahlerPotential := Expand[invarH2 + invarK2] / MP^2;
invarK3 := FullSimplify[Tr[kH.kH.kH]];
invarHK3 := FullSimplify[hL.kH.hR];
invarH2;
invarK2;
invarK3;
invarHK3;
kahlerPotential;

In[19]:= (* superpotential with parameter b *)
Wb := MP^(3 / 2) Exp[-kahlerPotential / (b)]
      ((g1 invarK3 - g2 invarHK3) / (2 Sqrt[2]))^(1 / 2);
WbShifted := Wb /. shiftAll;

(* EWSB equations *)
eqK12 := FullSimplify[D[WbShifted, K12] /. replaceAllFieldsWithZero]
eqK11 := FullSimplify[D[WbShifted, K11] /. replaceAllFieldsWithZero]
eqK29 := FullSimplify[D[WbShifted, K29] /. replaceAllFieldsWithZero]

```

```
In[24]:= eqK12
eqK11
eqK29
```

$$\text{Out[24]} = \left( e^{-\frac{MK1^2 + MK2^2 + MK9^2}{2bMP^2}} \left( 4\sqrt{15} g1 (-2MK2^2 (9MK1^2 + MK2^2) + 3b (3MK1^2 + MK2^2) MP^2) - \right. \right. \\ \left. \left. 3g2 MK9^2 (10MK1 MK2 + \sqrt{15} (-2MK2^2 + bMP^2)) \right) \right) / \\ \left( 4 \times 2^{1/4} b \sqrt{(60\sqrt{15} g1 MK2 (9MK1^2 + MK2^2) + 45g2 (5MK1 - \sqrt{15} MK2) MK9^2) \sqrt{MP}} \right)$$

$$\text{Out[25]} = \left( e^{-\frac{MK1^2 + MK2^2 + MK9^2}{2bMP^2}} (-8\sqrt{15} g1 MK1 MK2 (9MK1^2 + MK2^2 - 9bMP^2) + \right. \\ \left. 3g2 MK9^2 (2MK1 (-5MK1 + \sqrt{15} MK2) + 5bMP^2) \right) / \\ \left( 4 \times 2^{1/4} b \sqrt{(60\sqrt{15} g1 MK2 (9MK1^2 + MK2^2) + 45g2 (5MK1 - \sqrt{15} MK2) MK9^2) \sqrt{MP}} \right)$$

$$\text{Out[26]} = \left( e^{-\frac{MK1^2 + MK2^2 + MK9^2}{2bMP^2}} MK9 (-4\sqrt{15} g1 MK2 (9MK1^2 + MK2^2) + 3g2 (-5MK1 + \sqrt{15} MK2) (MK9^2 - bMP^2)) \right) / \\ \left( 2 \times 2^{1/4} b \sqrt{(60\sqrt{15} g1 MK2 (9MK1^2 + MK2^2) + 45g2 (5MK1 - \sqrt{15} MK2) MK9^2) \sqrt{MP}} \right)$$

```
In[27]:= numerators = Numerator[{eqK11, eqK12, eqK29}];
numerators
```

$$\text{Out[28]} = \left\{ -8\sqrt{15} g1 MK1 MK2 (9MK1^2 + MK2^2 - 9bMP^2) + 3g2 MK9^2 (2MK1 (-5MK1 + \sqrt{15} MK2) + 5bMP^2), \right. \\ 4\sqrt{15} g1 (-2MK2^2 (9MK1^2 + MK2^2) + 3b (3MK1^2 + MK2^2) MP^2) - \\ 3g2 MK9^2 (10MK1 MK2 + \sqrt{15} (-2MK2^2 + bMP^2)), \\ \left. MK9 (-4\sqrt{15} g1 MK2 (9MK1^2 + MK2^2) + 3g2 (-5MK1 + \sqrt{15} MK2) (MK9^2 - bMP^2)) \right\}$$

```
In[29]:= ewsbEqs := Thread[numerators == 0];
ewsbEqs
```

$$\text{Out[30]} = \left\{ -8\sqrt{15} g1 MK1 MK2 (9MK1^2 + MK2^2 - 9bMP^2) + 3g2 MK9^2 (2MK1 (-5MK1 + \sqrt{15} MK2) + 5bMP^2) == \right. \\ 0, 4\sqrt{15} g1 (-2MK2^2 (9MK1^2 + MK2^2) + 3b (3MK1^2 + MK2^2) MP^2) - \\ 3g2 MK9^2 (10MK1 MK2 + \sqrt{15} (-2MK2^2 + bMP^2)) == 0, \\ \left. MK9 (-4\sqrt{15} g1 MK2 (9MK1^2 + MK2^2) + 3g2 (-5MK1 + \sqrt{15} MK2) (MK9^2 - bMP^2)) == 0 \right\}$$

```
In[31]:= ewsbEqSolns := Simplify[Solve[ewsbEqs, {MK1, MK2, MK9}]]
ewsbEqSolns;
```

```

In[33]:= FullSimplify[ewsbEqSolns[[15]], Assumptions → {MP > 0}]
Out[33]= {MK1 → -((3 √b √g2 (2 g1 + g2) MP) / (4 √(108 g13 + 72 g12 g2 - 9 g1 g22 + g23))),
          MK2 → -((√15 √b √g2 (-6 g1 + g2) MP) / (4 √(108 g13 + 72 g12 g2 - 9 g1 g22 + g23))),
          MK9 → (3 √((b g1 (18 g1 - g2) (-6 g1 + g2)2 (2 g1 + g2) (36 g12 + 6 g1 g2 - g22)) /
                  (108 g13 + 72 g12 g2 - 9 g1 g22 + g23)) MP) /
          (√2 √((-6 g1 + g2)2 (36 g12 + 6 g1 g2 - g22)))}

In[34]:= FullSimplify[ewsbEqs /. ewsbEqSolns[[15]]]
Out[34]= {True, True, True}

In[35]:=
(* mass matrices *)
firstDerivs = D[WbShifted, #] & /@ Table[Symbol["K" <> ToString[i]], {i, 1, 34}];
(* firstDerivs *)

In[36]:= secondDerivs = Map[D[WbShifted, #][[1]], #][[2]] &,
          Table[{Symbol["K" <> ToString[i]], Symbol["K" <> ToString[j]]},
                {i, 1, 34}, {j, 1, 34}], {2}];
(* secondDerivs *)

In[37]:= prefactorforscalarmassssquared :=
          FullSimplify[Exp[kahlerPotential] /. shiftAll /. replaceAllFieldsWithZero /.
                      ewsbEqSolns[[15]]] /. b → 4; prefactorforscalarmassssquared
Out[37]= e3

In[38]:= massMatrix = secondDerivs /. replaceAllFieldsWithZero;

In[39]:= simplifiedMassMatrix = Simplify[massMatrix /. ewsbEqSolns[[15]], MP > 0];

In[40]:= massEigenvalues = Eigenvalues[simplifiedMassMatrix];

In[41]:= Tally[massEigenvalues];

```

---

Here are the eigenvalues and multiplicities for the scalar masses squared expressed in terms of g1 and g2 and the Planck mass MP:

```

In[42]:= tallyscalarmassssquared :=
          Simplify[Tally[prefactorforscalarmassssquared (massEigenvalues /. b → 4)2]];
          tallyscalarmassssquared
Out[42]= {{0, 15},
          {-((3 e3/2 g1 (-3 g1 + g2)2 MP2) / (√2 √g2 √(108 g13 + 72 g12 g2 - 9 g1 g22 + g23))), 8},
          {-((e3/2 (-36 g12 - 36 g1 g2 + g22)2 MP2) /

```

$$\begin{aligned}
& \left( 192 \sqrt{2} \, g_1 \sqrt{g_2} \sqrt{(108 g_1^3 + 72 g_1^2 g_2 - 9 g_1 g_2^2 + g_2^3)} \right), 6 \}, \\
& \left\{ - \left( \left( 3 e^{3/2} (36 g_1^2 + g_2^2)^2 \text{MP}^2 \right) / \left( 64 \sqrt{2} \, g_1 \sqrt{g_2} \sqrt{(108 g_1^3 + 72 g_1^2 g_2 - 9 g_1 g_2^2 + g_2^3)} \right) \right), 2 \right\}, \\
& \left\{ - \left( \left( e^{3/2} \text{MP}^2 \right. \right. \right. \\
& \quad \text{Root} \left[ -16\,048\,980\,806\,860\,800 \sqrt{3} \, g_1^{15} g_2^{11/2} \sqrt{(6 g_1 - g_2)^2 (36 g_1^2 + 6 g_1 g_2 - g_2^2)} \right. \\
& \quad \sqrt{(108 g_1^3 + 72 g_1^2 g_2 - 9 g_1 g_2^2 + g_2^3)} - 9\,807\,710\,493\,081\,600 \sqrt{3} \, g_1^{14} g_2^{13/2} \\
& \quad \sqrt{(6 g_1 - g_2)^2 (36 g_1^2 + 6 g_1 g_2 - g_2^2)} \sqrt{(108 g_1^3 + 72 g_1^2 g_2 - 9 g_1 g_2^2 + g_2^3)} + \\
& \quad 5\,944\,066\,965\,504\,000 \sqrt{3} \, g_1^{13} g_2^{15/2} \sqrt{(6 g_1 - g_2)^2 (36 g_1^2 + 6 g_1 g_2 - g_2^2)} \\
& \quad \sqrt{(108 g_1^3 + 72 g_1^2 g_2 - 9 g_1 g_2^2 + g_2^3)} + 1\,708\,919\,252\,582\,400 \sqrt{3} \, g_1^{12} g_2^{17/2} \\
& \quad \sqrt{(6 g_1 - g_2)^2 (36 g_1^2 + 6 g_1 g_2 - g_2^2)} \sqrt{(108 g_1^3 + 72 g_1^2 g_2 - 9 g_1 g_2^2 + g_2^3)} - \\
& \quad 9\,659\,108\,818\,944\,000 \sqrt{3} \, g_1^{11} g_2^{19/2} \sqrt{(6 g_1 - g_2)^2 (36 g_1^2 + 6 g_1 g_2 - g_2^2)} \\
& \quad \sqrt{(108 g_1^3 + 72 g_1^2 g_2 - 9 g_1 g_2^2 + g_2^3)} + 51\,597\,803\,520\,000 \sqrt{3} \, g_1^{10} g_2^{21/2} \\
& \quad \sqrt{(6 g_1 - g_2)^2 (36 g_1^2 + 6 g_1 g_2 - g_2^2)} \sqrt{(108 g_1^3 + 72 g_1^2 g_2 - 9 g_1 g_2^2 + g_2^3)} + \\
& \quad 33\,481\,241\,395\,200 \sqrt{3} \, g_1^9 g_2^{23/2} \sqrt{(6 g_1 - g_2)^2 (36 g_1^2 + 6 g_1 g_2 - g_2^2)} \\
& \quad \sqrt{(108 g_1^3 + 72 g_1^2 g_2 - 9 g_1 g_2^2 + g_2^3)} - 8\,121\,876\,480\,000 \sqrt{3} \, g_1^8 g_2^{25/2} \\
& \quad \sqrt{(6 g_1 - g_2)^2 (36 g_1^2 + 6 g_1 g_2 - g_2^2)} \sqrt{(108 g_1^3 + 72 g_1^2 g_2 - 9 g_1 g_2^2 + g_2^3)} + \\
& \quad 882\,258\,739\,200 \sqrt{3} \, g_1^7 g_2^{27/2} \sqrt{(6 g_1 - g_2)^2 (36 g_1^2 + 6 g_1 g_2 - g_2^2)} \\
& \quad \sqrt{(108 g_1^3 + 72 g_1^2 g_2 - 9 g_1 g_2^2 + g_2^3)} - \\
& \quad 48\,837\,427\,200 \sqrt{3} \, g_1^6 g_2^{29/2} \sqrt{(6 g_1 - g_2)^2 (36 g_1^2 + 6 g_1 g_2 - g_2^2)} \\
& \quad \sqrt{(108 g_1^3 + 72 g_1^2 g_2 - 9 g_1 g_2^2 + g_2^3)} + 1\,061\,683\,200 \sqrt{3} \, g_1^5 g_2^{31/2} \\
& \quad \sqrt{(6 g_1 - g_2)^2 (36 g_1^2 + 6 g_1 g_2 - g_2^2)} \sqrt{(108 g_1^3 + 72 g_1^2 g_2 - 9 g_1 g_2^2 + g_2^3)} + \\
& \quad (8\,358\,844\,170\,240 g_1^{13} g_2^3 + 14\,395\,787\,182\,080 g_1^{12} g_2^4 + 2\,321\,901\,158\,400 g_1^{11} \\
& \quad g_2^5 - 2\,824\,979\,742\,720 g_1^{10} g_2^6 + 309\,586\,821\,120 g_1^9 g_2^7 + 80\,621\,568\,000 \\
& \quad g_1^8 g_2^8 - 28\,784\,885\,760 g_1^7 g_2^9 + 4\,329\,676\,800 g_1^6 g_2^{10} - 376\,565\,760 g_1^5 \\
& \quad g_2^{11} + 19\,906\,560 g_1^4 g_2^{12} - 552\,960 g_1^3 g_2^{13}) \#1 + (-11\,520 \sqrt{3} \, g_1^3 g_2^{3/2} \\
& \quad \sqrt{(6 g_1 - g_2)^2 (36 g_1^2 + 6 g_1 g_2 - g_2^2)} \sqrt{(108 g_1^3 + 72 g_1^2 g_2 - 9 g_1 g_2^2 + \\
& \quad g_2^3)} - 2880 \sqrt{3} \, g_1^2 g_2^{5/2} \sqrt{(6 g_1 - g_2)^2 (36 g_1^2 + 6 g_1 g_2 - g_2^2)} \\
& \quad \sqrt{(108 g_1^3 + 72 g_1^2 g_2 - 9 g_1 g_2^2 + g_2^3)}) \#1^2 + \#1^3 \&, 1 \Big]^2 \Big) / \\
& \quad \left( 3\,686\,400 \sqrt{2} \, g_1^3 g_2^{7/2} (-6 g_1 + g_2)^2 (36 g_1^2 + 6 g_1 g_2 - g_2^2) \right. \\
& \quad \left. (108 g_1^3 + 72 g_1^2 g_2 - 9 g_1 g_2^2 + g_2^3)^{3/2} \right), 1 \}, \\
& \left\{ - \left( \left( e^{3/2} \text{MP}^2 \text{Root} \left[ -16\,048\,980\,806\,860\,800 \sqrt{3} \, g_1^{15} g_2^{11/2} \right. \right. \right. \\
& \quad \sqrt{(6 g_1 - g_2)^2 (36 g_1^2 + 6 g_1 g_2 - g_2^2)} \sqrt{(108 g_1^3 + 72 g_1^2 g_2 - 9 g_1 g_2^2 + g_2^3)} - \\
& \quad 9\,807\,710\,493\,081\,600 \sqrt{3} \, g_1^{14} g_2^{13/2} \sqrt{(6 g_1 - g_2)^2 (36 g_1^2 + 6 g_1 g_2 - g_2^2)} \\
& \quad \sqrt{(108 g_1^3 + 72 g_1^2 g_2 - 9 g_1 g_2^2 + g_2^3)} + 5\,944\,066\,965\,504\,000 \sqrt{3} \, g_1^{13} g_2^{15/2} \\
& \quad \sqrt{(6 g_1 - g_2)^2 (36 g_1^2 + 6 g_1 g_2 - g_2^2)} \sqrt{(108 g_1^3 + 72 g_1^2 g_2 - 9 g_1 g_2^2 + g_2^3)} + \\
& \quad 1\,708\,919\,252\,582\,400 \sqrt{3} \, g_1^{12} g_2^{17/2} \sqrt{(6 g_1 - g_2)^2 (36 g_1^2 + 6 g_1 g_2 - g_2^2)} \\
& \quad \sqrt{(108 g_1^3 + 72 g_1^2 g_2 - 9 g_1 g_2^2 + g_2^3)} - 9\,659\,108\,818\,944\,000 \sqrt{3} \, g_1^{11} g_2^{19/2} \\
& \quad \sqrt{(6 g_1 - g_2)^2 (36 g_1^2 + 6 g_1 g_2 - g_2^2)} \sqrt{(108 g_1^3 + 72 g_1^2 g_2 - 9 g_1 g_2^2 + g_2^3)} +
\end{aligned}$$

$$\begin{aligned}
& 51\,597\,803\,520\,000 \sqrt{3} \, g_1^{10} g_2^{21/2} \sqrt{\left((6g_1 - g_2)^2 (36g_1^2 + 6g_1g_2 - g_2^2)\right)} \\
& \sqrt{\left(108g_1^3 + 72g_1^2g_2 - 9g_1g_2^2 + g_2^3\right)} + 33\,481\,241\,395\,200 \sqrt{3} \, g_1^9 g_2^{23/2} \\
& \sqrt{\left((6g_1 - g_2)^2 (36g_1^2 + 6g_1g_2 - g_2^2)\right)} \sqrt{\left(108g_1^3 + 72g_1^2g_2 - 9g_1g_2^2 + g_2^3\right)} - \\
& 8\,121\,876\,480\,000 \sqrt{3} \, g_1^8 g_2^{25/2} \sqrt{\left((6g_1 - g_2)^2 (36g_1^2 + 6g_1g_2 - g_2^2)\right)} \\
& \sqrt{\left(108g_1^3 + 72g_1^2g_2 - 9g_1g_2^2 + g_2^3\right)} + 882\,258\,739\,200 \sqrt{3} \, g_1^7 g_2^{27/2} \\
& \sqrt{\left((6g_1 - g_2)^2 (36g_1^2 + 6g_1g_2 - g_2^2)\right)} \sqrt{\left(108g_1^3 + 72g_1^2g_2 - 9g_1g_2^2 + g_2^3\right)} - \\
& 48\,837\,427\,200 \sqrt{3} \, g_1^6 g_2^{29/2} \sqrt{\left((6g_1 - g_2)^2 (36g_1^2 + 6g_1g_2 - g_2^2)\right)} \\
& \sqrt{\left(108g_1^3 + 72g_1^2g_2 - 9g_1g_2^2 + g_2^3\right)} + 1\,061\,683\,200 \sqrt{3} \, g_1^5 g_2^{31/2} \\
& \sqrt{\left((6g_1 - g_2)^2 (36g_1^2 + 6g_1g_2 - g_2^2)\right)} \sqrt{\left(108g_1^3 + 72g_1^2g_2 - 9g_1g_2^2 + g_2^3\right)} + \\
& \left(8\,358\,844\,170\,240 g_1^{13} g_2^3 + 14\,395\,787\,182\,080 g_1^{12} g_2^4 + 2\,321\,901\,158\,400 \right. \\
& \quad \left. g_1^{11} g_2^5 - 2\,824\,979\,742\,720 g_1^{10} g_2^6 + 309\,586\,821\,120 g_1^9 g_2^7 + \right. \\
& \quad \left. 80\,621\,568\,000 g_1^8 g_2^8 - 28\,784\,885\,760 g_1^7 g_2^9 + 4\,329\,676\,800 g_1^6 \right. \\
& \quad \left. g_2^{10} - 376\,565\,760 g_1^5 g_2^{11} + 19\,906\,560 g_1^4 g_2^{12} - 552\,960 g_1^3 g_2^{13}\right) \#1 + \\
& \left(-11\,520 \sqrt{3} \, g_1^3 g_2^{3/2} \sqrt{\left((6g_1 - g_2)^2 (36g_1^2 + 6g_1g_2 - g_2^2)\right)} \right. \\
& \quad \left. \sqrt{\left(108g_1^3 + 72g_1^2g_2 - 9g_1g_2^2 + g_2^3\right)} - 2880 \sqrt{3} \right. \\
& \quad \left. g_1^2 g_2^{5/2} \sqrt{\left((6g_1 - g_2)^2 (36g_1^2 + 6g_1g_2 - g_2^2)\right)} \right. \\
& \quad \left. \sqrt{\left(108g_1^3 + 72g_1^2g_2 - 9g_1g_2^2 + g_2^3\right)} \right) \#1^2 + \#1^3 \&, 2\big]^2 \bigg) / \\
& \left(3\,686\,400 \sqrt{2} \, g_1^3 g_2^{7/2} (-6g_1 + g_2)^2 (36g_1^2 + 6g_1g_2 - g_2^2) \right. \\
& \quad \left. (108g_1^3 + 72g_1^2g_2 - 9g_1g_2^2 + g_2^3)^{3/2}\right), 1\big\}, \\
& \left\{-\left(\left(e^{3/2} \text{MP}^2 \text{Root}\left[-16\,048\,980\,806\,860\,800 \sqrt{3} \, g_1^{15} g_2^{11/2} \right.\right.\right. \\
& \quad \left.\left.\sqrt{\left((6g_1 - g_2)^2 (36g_1^2 + 6g_1g_2 - g_2^2)\right)} \sqrt{\left(108g_1^3 + 72g_1^2g_2 - 9g_1g_2^2 + g_2^3\right)} - \right.\right. \\
& \quad \left.\left.9\,807\,710\,493\,081\,600 \sqrt{3} \, g_1^{14} g_2^{13/2} \sqrt{\left((6g_1 - g_2)^2 (36g_1^2 + 6g_1g_2 - g_2^2)\right)} \right.\right. \\
& \quad \left.\left.\sqrt{\left(108g_1^3 + 72g_1^2g_2 - 9g_1g_2^2 + g_2^3\right)} + 5\,944\,066\,965\,504\,000 \sqrt{3} \, g_1^{13} g_2^{15/2} \right.\right. \\
& \quad \left.\left.\sqrt{\left((6g_1 - g_2)^2 (36g_1^2 + 6g_1g_2 - g_2^2)\right)} \sqrt{\left(108g_1^3 + 72g_1^2g_2 - 9g_1g_2^2 + g_2^3\right)} + \right.\right. \\
& \quad \left.\left.1\,708\,919\,252\,582\,400 \sqrt{3} \, g_1^{12} g_2^{17/2} \sqrt{\left((6g_1 - g_2)^2 (36g_1^2 + 6g_1g_2 - g_2^2)\right)} \right.\right. \\
& \quad \left.\left.\sqrt{\left(108g_1^3 + 72g_1^2g_2 - 9g_1g_2^2 + g_2^3\right)} - 965\,910\,881\,894\,400 \sqrt{3} \, g_1^{11} g_2^{19/2} \right.\right. \\
& \quad \left.\left.\sqrt{\left((6g_1 - g_2)^2 (36g_1^2 + 6g_1g_2 - g_2^2)\right)} \sqrt{\left(108g_1^3 + 72g_1^2g_2 - 9g_1g_2^2 + g_2^3\right)} + \right.\right. \\
& \quad \left.\left.51\,597\,803\,520\,000 \sqrt{3} \, g_1^{10} g_2^{21/2} \sqrt{\left((6g_1 - g_2)^2 (36g_1^2 + 6g_1g_2 - g_2^2)\right)} \right.\right. \\
& \quad \left.\left.\sqrt{\left(108g_1^3 + 72g_1^2g_2 - 9g_1g_2^2 + g_2^3\right)} + 33\,481\,241\,395\,200 \sqrt{3} \, g_1^9 g_2^{23/2} \right.\right. \\
& \quad \left.\left.\sqrt{\left((6g_1 - g_2)^2 (36g_1^2 + 6g_1g_2 - g_2^2)\right)} \sqrt{\left(108g_1^3 + 72g_1^2g_2 - 9g_1g_2^2 + g_2^3\right)} - \right.\right. \\
& \quad \left.\left.8\,121\,876\,480\,000 \sqrt{3} \, g_1^8 g_2^{25/2} \sqrt{\left((6g_1 - g_2)^2 (36g_1^2 + 6g_1g_2 - g_2^2)\right)} \right.\right. \\
& \quad \left.\left.\sqrt{\left(108g_1^3 + 72g_1^2g_2 - 9g_1g_2^2 + g_2^3\right)} + 882\,258\,739\,200 \sqrt{3} \, g_1^7 g_2^{27/2} \right.\right. \\
& \quad \left.\left.\sqrt{\left((6g_1 - g_2)^2 (36g_1^2 + 6g_1g_2 - g_2^2)\right)} \sqrt{\left(108g_1^3 + 72g_1^2g_2 - 9g_1g_2^2 + g_2^3\right)} - \right.\right. \\
& \quad \left.\left.48\,837\,427\,200 \sqrt{3} \, g_1^6 g_2^{29/2} \sqrt{\left((6g_1 - g_2)^2 (36g_1^2 + 6g_1g_2 - g_2^2)\right)} \right.\right. \\
& \quad \left.\left.\sqrt{\left(108g_1^3 + 72g_1^2g_2 - 9g_1g_2^2 + g_2^3\right)} + 1\,061\,683\,200 \sqrt{3} \, g_1^5 g_2^{31/2} \right.\right. \\
& \quad \left.\left.\sqrt{\left((6g_1 - g_2)^2 (36g_1^2 + 6g_1g_2 - g_2^2)\right)} \sqrt{\left(108g_1^3 + 72g_1^2g_2 - 9g_1g_2^2 + g_2^3\right)} + \right.\right. \\
& \quad \left.\left.8\,358\,844\,170\,240 g_1^{13} g_2^3 + 14\,395\,787\,182\,080 g_1^{12} g_2^4 + 2\,321\,901\,158\,400 \right.\right. \\
& \quad \left.\left. g_1^{11} g_2^5 - 2\,824\,979\,742\,720 g_1^{10} g_2^6 + 309\,586\,821\,120 g_1^9 g_2^7 + \right.\right.
\end{aligned}$$

$$\begin{aligned}
& 80\,621\,568\,000\,g_1^8\,g_2^8 - 28\,784\,885\,760\,g_1^7\,g_2^9 + 4\,329\,676\,800\,g_1^6\,g_2^{10} - 376\,565\,760\,g_1^5\,g_2^{11} + 19\,906\,560\,g_1^4\,g_2^{12} - 552\,960\,g_1^3\,g_2^{13} \Big) \#1 + \\
& \left( -11\,520\sqrt{3}\,g_1^3\,g_2^{3/2} \sqrt{(6\,g_1 - g_2)^2 (36\,g_1^2 + 6\,g_1\,g_2 - g_2^2)} \right. \\
& \quad \sqrt{(108\,g_1^3 + 72\,g_1^2\,g_2 - 9\,g_1\,g_2^2 + g_2^3)} - 2880\sqrt{3}\,g_1^2\,g_2^{5/2} \sqrt{(6\,g_1 - g_2)^2 (36\,g_1^2 + 6\,g_1\,g_2 - g_2^2)} \\
& \quad \left. \sqrt{(108\,g_1^3 + 72\,g_1^2\,g_2 - 9\,g_1\,g_2^2 + g_2^3)} \Big) \#1^2 + \#1^3 \&, 3 \Big)^2 \right) / \\
& \left( 3\,686\,400\sqrt{2}\,g_1^3\,g_2^{7/2} (-6\,g_1 + g_2)^2 (36\,g_1^2 + 6\,g_1\,g_2 - g_2^2) \right. \\
& \quad \left. (108\,g_1^3 + 72\,g_1^2\,g_2 - 9\,g_1\,g_2^2 + g_2^3)^{3/2} \right) \Big), 1 \Big\} \Big\}
\end{aligned}$$

Introducing the ratio  $r$  and the parameter  $f$ , and  $r$  as a series in  $f$  for small  $f$ , to solve for the VeVs

```
In[43]:= rnumerators = Simplify[Cancel[
  (Numerator[{eqK11 /. g2 -> r g1, eqK12 /. g2 -> r g1, eqK29 /. g2 -> r g1}]) / g1]];
rnumerators
```

```
Out[44]= {-72 Sqrt[15] MK1^3 MK2 - 30 MK1^2 MK9^2 r + 15 b MK9^2 MP^2 r +
  2 Sqrt[15] MK1 MK2 (-4 MK2^2 + 36 b MP^2 + 3 MK9^2 r), 36 Sqrt[15] MK1^2 (-2 MK2^2 + b MP^2) -
  30 MK1 MK2 MK9^2 r + Sqrt[15] (-8 MK2^4 - 3 b MK9^2 MP^2 r + 6 MK2^2 (2 b MP^2 + MK9^2 r)),
  MK9 (-36 Sqrt[15] MK1^2 MK2 - 15 MK1 (MK9^2 - b MP^2) r + Sqrt[15] MK2 (-4 MK2^2 + 3 (MK9^2 - b MP^2) r)) }
```

```
In[45]:= rnewnumerators = Collect[Simplify[
  Cancel[(Numerator[{eqK11 /. g2 -> r g1, eqK12 /. g2 -> r g1, eqK29 /. g2 -> r g1}]) /
  g1]], r, Simplify]
```

```
Out[45]= {-8 Sqrt[15] MK1 MK2 (9 MK1^2 + MK2^2 - 9 b MP^2) + 3 MK9^2 (-10 MK1^2 + 2 Sqrt[15] MK1 MK2 + 5 b MP^2) r,
  4 Sqrt[15] (-2 MK2^4 + 3 b MK2^2 MP^2 + 9 MK1^2 (-2 MK2^2 + b MP^2)) -
  3 MK9^2 (10 MK1 MK2 + Sqrt[15] (-2 MK2^2 + b MP^2)) r,
  -4 Sqrt[15] MK2 (9 MK1^2 + MK2^2) MK9 + 3 (-5 MK1 + Sqrt[15] MK2) MK9 (MK9^2 - b MP^2) r }
```

```
In[46]:= rewsbeqs := Thread[rnewnumerators == 0] /. b -> 4
```

```
In[47]:= rewsbeqs /. {MK1 -> M_K1, MK2 -> M_K2, MK9 -> M_K9, MP -> M_P}
```

```
Out[47]= {-8 Sqrt[15] M_K1 M_K2 (9 M_K1^2 + M_K2^2 - 36 M_P^2) + 3 r M_K9^2 (-10 M_K1^2 + 2 Sqrt[15] M_K1 M_K2 + 20 M_P^2) == 0,
  -3 r M_K9^2 (10 M_K1 M_K2 + Sqrt[15] (-2 M_K2^2 + 4 M_P^2)) + 4 Sqrt[15] (-2 M_K2^4 + 12 M_K2^2 M_P^2 + 9 M_K1^2 (-2 M_K2^2 + 4 M_P^2)) ==
  0, -4 Sqrt[15] M_K2 (9 M_K1^2 + M_K2^2) M_K9 + 3 r (-5 M_K1 + Sqrt[15] M_K2) M_K9 (M_K9^2 - 4 M_P^2) == 0 }
```

```
In[48]:= (* write ewsb equations and solutions in TeX for paper *)
```

In[49]:= **TeXForm[rewebeqs /. {MK1 → M<sub>K1</sub>, MK2 → M<sub>K2</sub>, MK9 → M<sub>K9</sub>, MP → M<sub>P</sub>}]**

Out[49]//TeXForm=

$$\begin{aligned} & \left( 3 r M_{\text{K9}}^2 \left( 2 \sqrt{15} M_{\text{K1}} M_{\text{K2}} - 10 M_{\text{K1}}^2 M_{\text{K2}}^2 - 8 \sqrt{15} M_{\text{K1}} M_{\text{K2}}^2 \right) - 10 M_{\text{K1}}^2 M_{\text{K2}}^2 \right. \\ & \quad \left. M_{\text{K1}}^2 + M_{\text{K2}}^2 - 36 M_{\text{P}}^2 \right) = 0, 4 \sqrt{15} \left( 9 M_{\text{K1}}^2 M_{\text{K2}}^2 - 12 M_{\text{K1}}^2 M_{\text{K2}}^2 M_{\text{P}}^2 - 2 M_{\text{K1}}^2 M_{\text{K2}}^2 M_{\text{P}}^2 \right. \\ & \quad \left. M_{\text{K9}}^2 \right) \left( 10 M_{\text{K1}} M_{\text{K2}} + \sqrt{15} \left( 4 M_{\text{P}}^2 - 2 M_{\text{K2}}^2 \right) \right) = 0, 3 r M_{\text{K9}} \left( \sqrt{15} M_{\text{K2}} - M_{\text{K1}} \right) \\ & \quad \left( M_{\text{K9}}^2 - 4 M_{\text{P}}^2 \right) - 4 \sqrt{15} M_{\text{K2}} M_{\text{K9}} \left( 9 M_{\text{K1}}^2 + M_{\text{K2}}^2 \right) = 0 \end{aligned}$$

In[50]:= **rsols = Simplify[Solve[Thread[rnewnumerators == 0], {MK1, MK2, MK9}], MP > 0];**  
**rsols;**

In[52]:= **rnewsol15 = {rsols[[15, 1]], rsols[[15, 2]],**  
**MK9 → -Sqrt[Cancel[Factor[(MK9 /. rsols[[15, 3]])^2]]] /. b → 4**

Out[52]= 
$$\left\{ \begin{aligned} \text{MK1} & \rightarrow \frac{3 \text{MP} \sqrt{r} (2 + r)}{2 \sqrt{108 + 72 r - 9 r^2 + r^3}}, \\ \text{MK2} & \rightarrow \frac{\sqrt{15} \text{MP} (-6 + r) \sqrt{r}}{2 \sqrt{108 + 72 r - 9 r^2 + r^3}}, \text{MK9} \rightarrow -3 \sqrt{2} \sqrt{-\frac{\text{MP}^2 (-18 + r) (2 + r)}{108 + 72 r - 9 r^2 + r^3}} \end{aligned} \right\}$$

In[53]:= **rsols15 := Simplify[rnewsol15, MP > 0]; rsols15**

Out[53]= 
$$\left\{ \begin{aligned} \text{MK1} & \rightarrow \frac{3 \text{MP} \sqrt{r} (2 + r)}{2 \sqrt{108 + 72 r - 9 r^2 + r^3}}, \\ \text{MK2} & \rightarrow \frac{\sqrt{15} \text{MP} (-6 + r) \sqrt{r}}{2 \sqrt{108 + 72 r - 9 r^2 + r^3}}, \text{MK9} \rightarrow -3 \sqrt{2} \text{MP} \sqrt{-\frac{(-18 + r) (2 + r)}{108 + 72 r - 9 r^2 + r^3}} \end{aligned} \right\}$$

In[54]:=

In[55]:= **Simplify[rnewsol15, MP > 0] /. {MK1 → M<sub>K1</sub>, MK2 → M<sub>K2</sub>, MK9 → M<sub>K9</sub>, MP → M<sub>P</sub>}**

Out[55]= 
$$\left\{ \begin{aligned} \text{M}_{\text{K1}} & \rightarrow \frac{3 \sqrt{r} (2 + r) \text{M}_{\text{P}}}{2 \sqrt{108 + 72 r - 9 r^2 + r^3}}, \\ \text{M}_{\text{K2}} & \rightarrow \frac{\sqrt{15} (-6 + r) \sqrt{r} \text{M}_{\text{P}}}{2 \sqrt{108 + 72 r - 9 r^2 + r^3}}, \text{M}_{\text{K9}} \rightarrow -3 \sqrt{2} \sqrt{-\frac{(-18 + r) (2 + r)}{108 + 72 r - 9 r^2 + r^3}} \text{M}_{\text{P}} \end{aligned} \right\}$$

In[56]:= **FullSimplify[rewebeqs /. rnewsol15]**

Out[56]= {True, True, True}



In[57]:= **TeXForm[Simplify[rnewsol15, MP > 0] /. {MK1 → M<sub>K1</sub>, MK2 → M<sub>K2</sub>, MK9 → M<sub>K9</sub>, MP → M<sub>P</sub>}]**

Out[57]//TeXForm=

$$\left\{ M_{\text{K1}} \rightarrow \frac{3 \sqrt{r} (r+2) M_P \{2 \sqrt{r^3-9 r^2+72 r+108}\}, M_{\text{K2}} \rightarrow \frac{\sqrt{15} (r-6) \sqrt{r} M_P \{2 \sqrt{r^3-9 r^2+72 r+108}\}, M_{\text{K9}} \rightarrow -3 \sqrt{2} \sqrt{-\frac{(r-18) (r+2)}{r^3-9 r^2+72 r+108}} M_P \right\}$$

In[58]:= **reqforf := (MK9 /. Simplify[rnewsol15, MP > 0])<sup>2</sup>/MP<sup>2</sup> == f<sup>2</sup>; reqforf**

Out[58]= 
$$-\frac{18 (-18+r) (2+r)}{108+72 r-9 r^2+r^3} == f^2$$

In[59]:= **r /. Simplify[Solve[reqforf, r]]**

Out[59]= 
$$\left\{ \frac{1}{f^2} \left( 3 (-2+f^2) + (3^{2/3} (-12-20 f^2+5 f^4)) \right) / \right. \\ \left. \left( 72+180 f^2-270 f^4+45 f^6+4 \sqrt{15} \sqrt{f^4 (-180-388 f^2+435 f^4-120 f^6+10 f^8)} \right)^{1/3} - \right. \\ \left. 3^{1/3} \left( 72+180 f^2-270 f^4+45 f^6+4 \sqrt{15} \sqrt{f^4 (-180-388 f^2+435 f^4-120 f^6+10 f^8)} \right)^{1/3} \right), \\ \frac{1}{2 f^2} \left( 6 (-2+f^2) - (i 3^{2/3} (-i+\sqrt{3}) (-12-20 f^2+5 f^4)) \right) / \\ \left( 72+180 f^2-270 f^4+45 f^6+4 \sqrt{15} \sqrt{f^4 (-180-388 f^2+435 f^4-120 f^6+10 f^8)} \right)^{1/3} + 3^{1/3} \\ (1-i \sqrt{3}) \\ \left( 72+180 f^2-270 f^4+45 f^6+4 \sqrt{15} \sqrt{f^4 (-180-388 f^2+435 f^4-120 f^6+10 f^8)} \right)^{1/3} \right), \\ \frac{1}{2 f^2} \left( 6 (-2+f^2) + (i 3^{2/3} (i+\sqrt{3}) (-12-20 f^2+5 f^4)) \right) / \\ \left( 72+180 f^2-270 f^4+45 f^6+4 \sqrt{15} \sqrt{f^4 (-180-388 f^2+435 f^4-120 f^6+10 f^8)} \right)^{1/3} + 3^{1/3} \\ (1+i \sqrt{3}) \\ \left( 72+180 f^2-270 f^4+45 f^6+4 \sqrt{15} \sqrt{f^4 (-180-388 f^2+435 f^4-120 f^6+10 f^8)} \right)^{1/3} \right\}$$

In[60]:= **rexpandedinf := Series[r /. Simplify[Solve[reqforf, r]], {f, 0, 3}]**

In[61]:= **rbigexpandedinf := Series[r /. Simplify[Solve[reqforf, r]], {f, 0, 13}]**

In[62]:= **rexpandedinf := Thread[r → Series[r /. Simplify[Solve[reqforf, r]], {f, 0, 3}]];**

In[63]:= **rexpandedinf**

Out[63]= 
$$\left\{ r \rightarrow -\frac{18}{f^2} - 7 + \frac{110 f^2}{9} + O[f]^4, r \rightarrow 18 - 12 f^2 + O[f]^4, r \rightarrow -2 - \frac{2 f^2}{9} + O[f]^4 \right\}$$

## Simplify

In[64]:= **ewsEqSolns15simp := {FullSimplify[ewsEqSolns[[15, 1]], Assumptions → {MP > 0}],  
FullSimplify[ewsEqSolns[[15, 2]], Assumptions → {MP > 0}],  
MK9 → Simplify[Sqrt[(MK9 /. FullSimplify[ewsEqSolns[[15]]])<sup>2</sup>], MP > 0]}**

In[65]:= **ewsbEqSolns15simp**

$$\text{Out[65]} = \left\{ \begin{aligned} \text{MK1} &\rightarrow - \left( \left( 3 \sqrt{b} \sqrt{g2} (2 g1 + g2) \text{MP} \right) / \left( 4 \sqrt{(108 g1^3 + 72 g1^2 g2 - 9 g1 g2^2 + g2^3)} \right) \right), \\ \text{MK2} &\rightarrow - \left( \left( \sqrt{15} \sqrt{b} \sqrt{g2} (-6 g1 + g2) \text{MP} \right) / \left( 4 \sqrt{(108 g1^3 + 72 g1^2 g2 - 9 g1 g2^2 + g2^3)} \right) \right), \\ \text{MK9} &\rightarrow \frac{3 \sqrt{\frac{b g1 (18 g1 - g2) (2 g1 + g2)}{108 g1^3 + 72 g1^2 g2 - 9 g1 g2^2 + g2^3}} \text{MP}}{\sqrt{2}} \end{aligned} \right\}$$

In[66]:= **FullSimplify[ewsbEqs /. ewsbEqSolns15simp]**

Out[66]= {True, True, True}

In[67]:= **ewsbEqSolns15simp4 := ewsbEqSolns15simp /. b -> 4;**

In[68]:= **ewsbEqSolns15simp4**

$$\text{Out[68]} = \left\{ \begin{aligned} \text{MK1} &\rightarrow - \left( \left( 3 \sqrt{g2} (2 g1 + g2) \text{MP} \right) / \left( 2 \sqrt{(108 g1^3 + 72 g1^2 g2 - 9 g1 g2^2 + g2^3)} \right) \right), \\ \text{MK2} &\rightarrow - \left( \left( \sqrt{15} \sqrt{g2} (-6 g1 + g2) \text{MP} \right) / \left( 2 \sqrt{(108 g1^3 + 72 g1^2 g2 - 9 g1 g2^2 + g2^3)} \right) \right), \\ \text{MK9} &\rightarrow 3 \sqrt{2} \sqrt{(g1 (18 g1 - g2) (2 g1 + g2)) / (108 g1^3 + 72 g1^2 g2 - 9 g1 g2^2 + g2^3)} \text{MP} \end{aligned} \right\}$$

In[69]:= **FullSimplify[ewsbEqs /. b -> 4 /. ewsbEqSolns15simp4]**

Out[69]= {True, True, True}

In[70]:= **TeXForm[ewsbEqSolns15simp4 /. {MK1 -> M\_K1, MK2 -> M\_K2, MK9 -> M\_K9, MP -> M\_P}]**

Out[70]/TeXForm=

$$\left\{ \begin{aligned} \text{M}_{\text{K1}} &\rightarrow - \frac{3 \sqrt{g2} (2 g1 + g2) \text{M}_P}{2 \sqrt{(108 g1^3 + 72 g1^2 g2 - 9 g1 g2^2 + g2^3)}}, \text{M}_{\text{K2}} \rightarrow - \frac{\sqrt{15} \sqrt{g2} (-6 g1 + g2) \text{M}_P}{2 \sqrt{(108 g1^3 + 72 g1^2 g2 - 9 g1 g2^2 + g2^3)}}, \\ \text{M}_{\text{K9}} &\rightarrow 3 \sqrt{2} \sqrt{\frac{g1 (18 g1 - g2) (2 g1 + g2)}{108 g1^3 + 72 g1^2 g2 - 9 g1 g2^2 + g2^3}} \text{M}_P \end{aligned} \right\}$$

## Values of the VeVs $M_{K1}$ etc in terms of the three possible values for $r$ in terms of $f$

In[71]:=

**rsols15 /. rexpandedinf**

$$\text{Out[71]} = \left\{ \begin{aligned} \text{MK1} &\rightarrow - \frac{3 \text{MP}}{2} + \frac{13 \text{MP} f^2}{24} - \frac{391 \text{MP} f^4}{1728} + O[f]^6, \\ \text{MK2} &\rightarrow - \frac{\sqrt{15} \text{MP}}{2} - \frac{1}{8} \left( \sqrt{\frac{5}{3}} \text{MP} \right) f^2 + \frac{115}{576} \sqrt{\frac{5}{3}} \text{MP} f^4 + O[f]^6, \text{MK9} \rightarrow -\text{MP} f + O[f]^7 \end{aligned} \right\}$$

```
In[72]:= Normal[Simplify[Table[rsols15[[i]] /. rexpandedinf[[j]], {j, 3}, {i, 3}]]]
```

$$\text{Out[72]} = \left\{ \left\{ \text{MK1} \rightarrow -\frac{3 \text{ MP}}{2} + \frac{13 f^2 \text{ MP}}{24} - \frac{391 f^4 \text{ MP}}{1728}, \text{MK2} \rightarrow -\frac{\sqrt{15} \text{ MP}}{2} - \frac{1}{8} \sqrt{\frac{5}{3}} f^2 \text{ MP} + \frac{115}{576} \sqrt{\frac{5}{3}} f^4 \text{ MP}, \right. \right.$$

$$\left. \text{MK9} \rightarrow -f \text{ MP} \right\}, \left\{ \text{MK1} \rightarrow \frac{\sqrt{15} \text{ MP}}{2} + \frac{f^2 \text{ MP}}{2 \sqrt{15}}, \text{MK2} \rightarrow \frac{3 \text{ MP}}{2} - \frac{f^2 \text{ MP}}{2}, \text{MK9} \rightarrow -f \text{ MP} \right\},$$

$$\left\{ \text{MK1} \rightarrow -\frac{f^2 \text{ MP}}{6 \sqrt{10}}, \text{MK2} \rightarrow -\sqrt{6} \text{ MP} + \frac{f^2 \text{ MP}}{2 \sqrt{6}}, \text{MK9} \rightarrow -f \text{ MP} \right\} \}$$

```
In[73]:= (* solutions in TeX for paper *)
```

```
In[74]:= TeXForm[
  Normal[Simplify[Table[rsols15[[i]] /. rexpandedinf[[j]], {j, 3}, {i, 3}]]] /.
  {MK1 -> M_K1, MK2 -> M_K2, MK9 -> M_K9, MP -> M_P}]
```

```
Out[74]//TeXForm=
```

```
\left\{\left\{M_{\text{K1}}\right\}\rightarrow -\frac{391 f^4 M_P}{1728}+\frac{13 f^2 M_P}{24}-\frac{f^2 M_P}{2},M_{\text{K2}}\right\}\rightarrow \frac{115}{576} \sqrt{\frac{5}{3}} f^4 M_P-\frac{1}{8} \sqrt{\frac{5}{3}} f^2 M_P-\frac{\sqrt{15} M_P}{2},M_{\text{K9}}\right\}\rightarrow -f M_P\right\},\left\{M_{\text{K1}}\right\}\rightarrow \frac{f^2 M_P}{2 \sqrt{15}}+\frac{\sqrt{15} M_P}{2},M_{\text{K2}}\right\}\rightarrow \frac{3 M_P}{2}-\frac{f^2 M_P}{2},M_{\text{K9}}\right\}\rightarrow -f M_P\right\},\left\{M_{\text{K1}}\right\}\rightarrow -\frac{f^2 M_P}{6 \sqrt{10}},M_{\text{K2}}\right\}\rightarrow -\sqrt{6} M_P+\frac{f^2 M_P}{2 \sqrt{6}},M_{\text{K9}}\right\}\rightarrow -f M_P\right\}\right\}
```

## The Vector Boson masses using the VeVs, as expanded in a series for small f

```
In[75]:= vecfromkH := Simplify[Tr[(vectorBosons.kH - kH.vectorBosons).
  (vectorBosons.kH - kH.vectorBosons)]] /. shiftAll
```

```
In[76]:= vecfromhLhR := Simplify[hL.vectorBosons.vectorBosons.hR] /. shiftAll
```

```
In[77]:= vecmass := g52 (-vecfromkH + vecfromhLhR);
```

```
In[78]:= justvecmass = vecmass /. replaceAllFieldsWithZero;
```

```
In[79]:= justvecmass;
```

```
In[80]:= TimeUsed[]
```

```
Out[80]= 162.404
```

```
In[81]:= secondDerivforvecbosons :=
  Map[D[justvecmass, #[[1]], #[[2]]] &, Table[{Symbol["V" <> ToString[i]],
    Symbol["V" <> ToString[j]]}, {i, 1, 24}, {j, 1, 24}], {2}];
```

```
In[82]:= Eigenvalues[secondDerivforvecbosons];
```

In[83]:= **Tally[Eigenvalues[secondDerivforvecbosons]]**

$$\text{Out[83]} = \left\{ \{0, 9\}, \left\{ \frac{4}{3} \left( 3 \text{MK1}^2 + 2 \sqrt{15} \text{MK1 MK2} + 5 \text{MK2}^2 \right) g_5^2, 6 \right\}, \left\{ \frac{8}{5} \text{MK9}^2 g_5^2, 1 \right\}, \right. \\ \left. \left\{ \left( 16 \text{MK1}^2 + \text{MK9}^2 \right) g_5^2, 2 \right\}, \left\{ \frac{1}{3} \left( 12 \text{MK1}^2 - 8 \sqrt{15} \text{MK1 MK2} + 20 \text{MK2}^2 + 3 \text{MK9}^2 \right) g_5^2, 6 \right\} \right\}$$

In[84]:= **ewsEqSolns15simp4**

$$\text{Out[84]} = \left\{ \text{MK1} \rightarrow - \left( \left( 3 \sqrt{g_2} \left( 2 g_1 + g_2 \right) \text{MP} \right) / \left( 2 \sqrt{\left( 108 g_1^3 + 72 g_1^2 g_2 - 9 g_1 g_2^2 + g_2^3 \right)} \right) \right), \right. \\ \text{MK2} \rightarrow - \left( \left( \sqrt{15} \sqrt{g_2} \left( -6 g_1 + g_2 \right) \text{MP} \right) / \left( 2 \sqrt{\left( 108 g_1^3 + 72 g_1^2 g_2 - 9 g_1 g_2^2 + g_2^3 \right)} \right) \right), \\ \left. \text{MK9} \rightarrow 3 \sqrt{2} \sqrt{\left( \left( g_1 \left( 18 g_1 - g_2 \right) \left( 2 g_1 + g_2 \right) \right) / \left( 108 g_1^3 + 72 g_1^2 g_2 - 9 g_1 g_2^2 + g_2^3 \right) \right) \text{MP}} \right\}$$

In[85]:= **vecmasseswithr := Factor[Simplify[**

**Tally[Eigenvalues[secondDerivforvecbosons]] /. ewsEqSolns15simp4 /. g2 -> r g1]]**

In[86]:= **vecmasseswithr**

$$\text{Out[86]} = \left\{ \{0, 9\}, \left\{ \frac{64 \text{MP}^2 (-3 + r)^2 r g_5^2}{108 + 72 r - 9 r^2 + r^3}, 6 \right\}, \right. \\ \left\{ -\frac{144 \text{MP}^2 (-18 + r) (2 + r) g_5^2}{5 (108 + 72 r - 9 r^2 + r^3)}, 1 \right\}, \left\{ \frac{18 \text{MP}^2 (2 + r) (18 + 3 r + 2 r^2) g_5^2}{108 + 72 r - 9 r^2 + r^3}, 2 \right\}, \\ \left. \left\{ \left( 2 \text{MP}^2 (-18 + r) (-18 - 45 r + 2 r^2) g_5^2 \right) / (108 + 72 r - 9 r^2 + r^3), 6 \right\} \right\}$$

In[87]:= **vecmasseswithr /. rexpandedinf[[1]]**

$$\text{Out[87]} = \left\{ \{0, 9\}, \left\{ 64 \text{MP}^2 g_5^2 - \frac{32}{3} \left( \text{MP}^2 g_5^2 \right) f^2 - \frac{80}{27} \left( \text{MP}^2 g_5^2 \right) f^4 + \text{O}[f]^6, 6 \right\}, \right. \\ \left\{ \frac{8}{5} \text{MP}^2 g_5^2 f^2 + \text{O}[f]^8, 1 \right\}, \left\{ 36 \text{MP}^2 g_5^2 - 25 \left( \text{MP}^2 g_5^2 \right) f^2 + \frac{140}{9} \text{MP}^2 g_5^2 f^4 + \text{O}[f]^6, 2 \right\}, \\ \left. \left\{ 4 \text{MP}^2 g_5^2 + 7 \text{MP}^2 g_5^2 f^2 - \frac{20}{9} \left( \text{MP}^2 g_5^2 \right) f^4 + \text{O}[f]^6, 6 \right\} \right\}$$

In[88]:= **vecmasseswithr /. rexpandedinf[[2]]**

$$\text{Out[88]} = \left\{ \{0, 9\}, \left\{ 60 \text{MP}^2 g_5^2 - 16 \left( \text{MP}^2 g_5^2 \right) f^2 + \text{O}[f]^4, 6 \right\}, \left\{ \frac{8}{5} \text{MP}^2 g_5^2 f^2 + \text{O}[f]^4, 1 \right\}, \right. \\ \left. \left\{ 60 \text{MP}^2 g_5^2 + 9 \text{MP}^2 g_5^2 f^2 + \text{O}[f]^4, 2 \right\}, \left\{ \text{MP}^2 g_5^2 f^2 + \text{O}[f]^4, 6 \right\} \right\}$$

In[89]:= **vecmasseswithr /. rexpandedinf[[3]]**

$$\text{Out[89]} = \left\{ \{0, 9\}, \left\{ 40 \text{MP}^2 g_5^2 - \frac{16}{3} \left( \text{MP}^2 g_5^2 \right) f^2 + \text{O}[f]^4, 6 \right\}, \left\{ \frac{8}{5} \text{MP}^2 g_5^2 f^2 + \text{O}[f]^4, 1 \right\}, \right. \\ \left. \left\{ \text{MP}^2 g_5^2 f^2 + \text{O}[f]^4, 2 \right\}, \left\{ 40 \text{MP}^2 g_5^2 - 7 \left( \text{MP}^2 g_5^2 \right) f^2 + \text{O}[f]^4, 6 \right\} \right\}$$

In[90]:= **Normal[vecmasseswithr /. rexpandedinf[[1]]] /. MP → M<sub>P</sub>**

$$\text{Out[90]} = \left\{ \{0, 9\}, \left\{ 64 g_5^2 M_P^2 - \frac{32}{3} f^2 g_5^2 M_P^2 - \frac{80}{27} f^4 g_5^2 M_P^2, 6 \right\}, \left\{ \frac{8}{5} f^2 g_5^2 M_P^2, 1 \right\}, \right. \\ \left. \left\{ 36 g_5^2 M_P^2 - 25 f^2 g_5^2 M_P^2 + \frac{140}{9} f^4 g_5^2 M_P^2, 2 \right\}, \left\{ 4 g_5^2 M_P^2 + 7 f^2 g_5^2 M_P^2 - \frac{20}{9} f^4 g_5^2 M_P^2, 6 \right\} \right\}$$

In[91]:= **Normal[vecmasseswithr /. rexpandedinf[[2]]] /. MP → M<sub>P</sub>**

$$\text{Out[91]} = \left\{ \{0, 9\}, \left\{ 60 g_5^2 M_P^2 - 16 f^2 g_5^2 M_P^2, 6 \right\}, \left\{ \frac{8}{5} f^2 g_5^2 M_P^2, 1 \right\}, \left\{ 60 g_5^2 M_P^2 + 9 f^2 g_5^2 M_P^2, 2 \right\}, \left\{ f^2 g_5^2 M_P^2, 6 \right\} \right\}$$

In[92]:= **Normal[vecmasseswithr /. rexpandedinf[[3]]] /. MP → M<sub>P</sub>**

$$\text{Out[92]} = \left\{ \{0, 9\}, \left\{ 40 g_5^2 M_P^2 - \frac{16}{3} f^2 g_5^2 M_P^2, 6 \right\}, \left\{ \frac{8}{5} f^2 g_5^2 M_P^2, 1 \right\}, \left\{ f^2 g_5^2 M_P^2, 2 \right\}, \left\{ 40 g_5^2 M_P^2 - 7 f^2 g_5^2 M_P^2, 6 \right\} \right\}$$

In[93]:= **vecm1 = TeXForm[Normal[vecmasseswithr /. rexpandedinf[[1]]] /. MP → M<sub>P</sub>];**

**vecm2 = TeXForm[Normal[vecmasseswithr /. rexpandedinf[[2]]] /. MP → M<sub>P</sub>];**

**vecm3 = TeXForm[Normal[vecmasseswithr /. rexpandedinf[[3]]] /. MP → M<sub>P</sub>];**

In[96]:= **(\* solutions in TeX for paper \*)**

In[97]:= **vecm1**

Out[97]//TeXForm=

$$\left( \begin{array}{cc} 0 & 9 \\ -\frac{80}{27} g_5^2 M_P^2 f^4 - \frac{32}{3} g_5^2 M_P^2 f^2 + 64 g_5^2 M_P^2 & 6 \\ \frac{8}{5} f^2 g_5^2 M_P^2 & 1 \\ \frac{140}{9} g_5^2 M_P^2 f^4 - 25 g_5^2 M_P^2 f^2 + 36 g_5^2 M_P^2 & 2 \\ -\frac{20}{9} g_5^2 M_P^2 f^4 + 7 g_5^2 M_P^2 f^2 + 40 g_5^2 M_P^2 & 6 \end{array} \right)$$

In[98]:= **vecm2**

Out[98]//TeXForm=

$$\left( \begin{array}{cc} 0 & 9 \\ 60 g_5^2 M_P^2 - 16 f^2 g_5^2 M_P^2 & 6 \\ \frac{8}{5} f^2 g_5^2 M_P^2 & 1 \\ 9 f^2 g_5^2 M_P^2 + 60 g_5^2 M_P^2 & 2 \\ f^2 g_5^2 M_P^2 & 6 \end{array} \right)$$

In[99]:= **vecm3**

Out[99]//TeXForm=

```
\left(
\begin{array}{cc}
0 & 9 \\\
40 g_5^2 M_P^2 - \frac{16}{3} f^2 g_5^2 M_P^2 & 6 \\\
\frac{8}{5} f^2 g_5^2 M_P^2 & 1 \\\
f^2 g_5^2 M_P^2 & 2 \\\
40 g_5^2 M_P^2 - 7 f^2 g_5^2 M_P^2 & 6 \\\
\end{array}
\right)
```

In[100]:= **TimeUsed[]**

Out[100]= 177.936

## Results for scalar mass matrix as a function of $r$ and $g_1$

In[101]:= **Normal[rexpandedinf[[3]]]**

Out[101]=  $r \rightarrow -2 - \frac{2 f^2}{9}$

In[102]:= **caallthistally := Cancel[Simplify[ tallyscalarmasssquaredeigs /. g2 → r g1 ]];**

In[103]:= **rbigtoof := FullSimplify[Thread[r → rbigexpandedinf]]; rbigtoof[[3]]**

Out[103]=  $r \rightarrow -2 - \frac{2 f^2}{9} - \frac{29 f^4}{405} - \frac{887 f^6}{36450} - \frac{5689 f^8}{656100} - \frac{316613 f^{10}}{98415000} - \frac{10934171 f^{12}}{8857350000} + O[f]^{14}$

In[104]:= **radicaltally := ToRadicals[caallthistally]**

The lowest mass for three neutral masses in the scalar mass matrix is the Higgs mass and it can be defined as  $M_H = h M_P$ . First we expand as a series for small  $f$

In[105]:= **scalarmassesfromf3 = FullSimplify[Series[radicaltally /. rbigtoof[[3]], {f, 0, 5}]];**  
**scalarmassesfromf3**

Out[106]=  $\left\{ \{0, 15\}, \right.$

$$\left\{ \frac{15 \sqrt{5} e^{3/2} \sqrt{-g_1^3} M_P^2}{8 \sqrt{-g_1}} - \frac{\left( \sqrt{5} e^{3/2} \sqrt{-g_1^3} M_P^2 \right) f^2}{4 \sqrt{-g_1}} - \frac{53 \left( e^{3/2} \sqrt{-g_1^3} M_P^2 \right) f^4}{576 \left( \sqrt{5} \sqrt{-g_1} \right)} + O[f]^6, 8 \right\},$$

$$\left\{ \frac{5 \sqrt{5} e^{3/2} \sqrt{-g_1^3} M_P^2}{24 \sqrt{-g_1}} + \frac{5 \sqrt{5} e^{3/2} \sqrt{-g_1^3} M_P^2 f^2}{108 \sqrt{-g_1}} + \frac{245 \sqrt{5} e^{3/2} \sqrt{-g_1^3} M_P^2 f^4}{15552 \sqrt{-g_1}} + O[f]^6, 6 \right\},$$

$$\begin{aligned}
& \left\{ \frac{15 \sqrt{5} \mathbf{e}^{3/2} \sqrt{-\mathbf{g}1^3} \mathbf{MP}^2}{8 \sqrt{-\mathbf{g}1}} - \frac{\left( \sqrt{5} \mathbf{e}^{3/2} \sqrt{-\mathbf{g}1^3} \mathbf{MP}^2 \right) \mathbf{f}^2}{3 \sqrt{-\mathbf{g}1}} - \frac{43 \left( \sqrt{5} \mathbf{e}^{3/2} \sqrt{-\mathbf{g}1^3} \mathbf{MP}^2 \right) \mathbf{f}^4}{1728 \sqrt{-\mathbf{g}1}} + \mathcal{O}[\mathbf{f}]^6, 2 \right\}, \\
& \left\{ \mathbf{e}^{3/2} \left( 13 \mathbf{g}1^{16} + \sqrt{3} (-\mathbf{g}1)^{7/2} \mathbf{g}1 \sqrt{-\mathbf{g}1^3} \sqrt{\mathbf{g}1^4} \left( -18 \sqrt{3} (-\mathbf{g}1)^{41/2} \sqrt{-\mathbf{g}1^3} \sqrt{\mathbf{g}1^4} + 35 \right. \right. \right. \\
& \quad \left. \left. \left. \sqrt{-\mathbf{g}1^{48}} \right)^{1/3} + \left( -18 \sqrt{3} (-\mathbf{g}1)^{41/2} \sqrt{-\mathbf{g}1^3} \sqrt{\mathbf{g}1^4} + 35 \sqrt{-\mathbf{g}1^{48}} \right)^{2/3} \right)^2 \mathbf{MP}^2 \right) / \\
& \quad \left( 8 \sqrt{5} (-\mathbf{g}1)^{27/2} \sqrt{-\mathbf{g}1^3} \left( -18 \sqrt{3} (-\mathbf{g}1)^{41/2} \sqrt{-\mathbf{g}1^3} \sqrt{\mathbf{g}1^4} + 35 \sqrt{-\mathbf{g}1^{48}} \right)^{2/3} \right) - \\
& \quad \left( \left( \sqrt{5} \mathbf{e}^{3/2} \mathbf{g}1^{23} \left( 17\,903 (-\mathbf{g}1)^{81/2} \sqrt{-\mathbf{g}1^3} + 12\,848 \sqrt{3} \mathbf{g}1^{16} \sqrt{\mathbf{g}1^4} \sqrt{-\mathbf{g}1^{48}} - \right. \right. \right. \\
& \quad \left. \left. \left. 1766 \sqrt{3} \mathbf{g}1^{32} \sqrt{\mathbf{g}1^4} \left( -18 \sqrt{3} (-\mathbf{g}1)^{41/2} \sqrt{-\mathbf{g}1^3} \sqrt{\mathbf{g}1^4} + 35 \sqrt{-\mathbf{g}1^{48}} \right)^{1/3} - 7307 \right. \right. \right. \\
& \quad \left. \left. \left. (-\mathbf{g}1)^{17/2} \sqrt{-\mathbf{g}1^3} \sqrt{-\mathbf{g}1^{48}} \left( -18 \sqrt{3} (-\mathbf{g}1)^{41/2} \sqrt{-\mathbf{g}1^3} \sqrt{\mathbf{g}1^4} + 35 \sqrt{-\mathbf{g}1^{48}} \right)^{1/3} + \right. \right. \right. \\
& \quad \left. \left. \left. 253 (-\mathbf{g}1)^{49/2} \sqrt{-\mathbf{g}1^3} \left( -18 \sqrt{3} (-\mathbf{g}1)^{41/2} \sqrt{-\mathbf{g}1^3} \sqrt{\mathbf{g}1^4} + 35 \sqrt{-\mathbf{g}1^{48}} \right)^{2/3} + \right. \right. \right. \\
& \quad \left. \left. \left. 1260 \sqrt{3} \sqrt{\mathbf{g}1^4} \sqrt{-\mathbf{g}1^{48}} \left( -18 \sqrt{3} (-\mathbf{g}1)^{41/2} \sqrt{-\mathbf{g}1^3} \sqrt{\mathbf{g}1^4} + 35 \sqrt{-\mathbf{g}1^{48}} \right)^{2/3} \right) \mathbf{MP}^2 \right) \right) \\
& \quad \left. \mathbf{f}^2 \right) / \left( 9 \left( -18 \sqrt{3} (-\mathbf{g}1)^{41/2} \sqrt{-\mathbf{g}1^3} \sqrt{\mathbf{g}1^4} + 35 \sqrt{-\mathbf{g}1^{48}} \right)^{8/3} \right) - \\
& \quad \left( \left( \mathbf{e}^{3/2} (-\mathbf{g}1)^{141/2} \left( -10\,457\,821\,477 \mathbf{g}1^{44} + 6\,307\,878\,046 \sqrt{3} (-\mathbf{g}1)^{33/2} \sqrt{-\mathbf{g}1^3} \sqrt{\mathbf{g}1^4} \sqrt{-\mathbf{g}1^{48}} + \right. \right. \right. \\
& \quad \left. \left. \left. 2\,128\,213\,604 \sqrt{3} (-\mathbf{g}1)^{65/2} \sqrt{-\mathbf{g}1^3} \sqrt{\mathbf{g}1^4} \right. \right. \right. \\
& \quad \left. \left( -18 \sqrt{3} (-\mathbf{g}1)^{41/2} \sqrt{-\mathbf{g}1^3} \sqrt{\mathbf{g}1^4} + 35 \sqrt{-\mathbf{g}1^{48}} \right)^{1/3} - 2\,001\,760\,259 \mathbf{g}1^{12} \right. \\
& \quad \left. \sqrt{-\mathbf{g}1^{48}} \left( -18 \sqrt{3} (-\mathbf{g}1)^{41/2} \sqrt{-\mathbf{g}1^3} \sqrt{\mathbf{g}1^4} + 35 \sqrt{-\mathbf{g}1^{48}} \right)^{1/3} - 653\,131\,949 \mathbf{g}1^{28} \right. \\
& \quad \left. \left( -18 \sqrt{3} (-\mathbf{g}1)^{41/2} \sqrt{-\mathbf{g}1^3} \sqrt{\mathbf{g}1^4} + 35 \sqrt{-\mathbf{g}1^{48}} \right)^{2/3} + 88\,620\,840 \sqrt{3} \sqrt{-\mathbf{g}1} \sqrt{-\mathbf{g}1^3} \right. \\
& \quad \left. \left. \left. \sqrt{\mathbf{g}1^4} \sqrt{-\mathbf{g}1^{48}} \left( -18 \sqrt{3} (-\mathbf{g}1)^{41/2} \sqrt{-\mathbf{g}1^3} \sqrt{\mathbf{g}1^4} + 35 \sqrt{-\mathbf{g}1^{48}} \right)^{2/3} \right) \mathbf{MP}^2 \right) \mathbf{f}^4 \right) / \\
& \quad \left( 5184 \left( \sqrt{5} \sqrt{-\mathbf{g}1^3} \left( -18 \sqrt{3} (-\mathbf{g}1)^{41/2} \sqrt{-\mathbf{g}1^3} \sqrt{\mathbf{g}1^4} + 35 \sqrt{-\mathbf{g}1^{48}} \right)^{14/3} \right) \right) + \\
& \quad \mathcal{O}[\mathbf{f}]^6, 1 \Big\}, \\
& \left\{ - \left( \mathbf{e}^{3/2} \left( -13 (-\mathbf{i} + \sqrt{3}) \mathbf{g}1^{16} + 2 \mathbf{i} \sqrt{3} (-\mathbf{g}1)^{9/2} \sqrt{-\mathbf{g}1^3} \sqrt{\mathbf{g}1^4} \right. \right. \right. \\
& \quad \left. \left. \left. \left( -18 \sqrt{3} (-\mathbf{g}1)^{41/2} \sqrt{-\mathbf{g}1^3} \sqrt{\mathbf{g}1^4} + 35 \sqrt{-\mathbf{g}1^{48}} \right)^{1/3} + \right. \right. \right.
\end{aligned}$$

$$\begin{aligned}
& \left( (\mathbf{i} + \sqrt{3}) \left( -18 \sqrt{3} (-\mathbf{g}1)^{41/2} \sqrt{-\mathbf{g}1^3} \sqrt{\mathbf{g}1^4} + 35 \sqrt{-\mathbf{g}1^{48}} \right)^{2/3} \right)^2 \text{MP}^2 \Bigg) / \\
& \left( 32 \left( \sqrt{5} (-\mathbf{g}1)^{27/2} \sqrt{-\mathbf{g}1^3} \left( -18 \sqrt{3} (-\mathbf{g}1)^{41/2} \sqrt{-\mathbf{g}1^3} \sqrt{\mathbf{g}1^4} + 35 \sqrt{-\mathbf{g}1^{48}} \right)^{2/3} \right) \right) \Bigg) - \\
& \left( \left( \sqrt{5} \mathbf{e}^{3/2} (-\mathbf{g}1)^{5/2} \left( 58 (-3 \mathbf{i} + \sqrt{3}) (-\mathbf{g}1)^{73/2} \sqrt{-\mathbf{g}1^3} \sqrt{\mathbf{g}1^4} + \right. \right. \right. \\
& \quad 601 \mathbf{i} (\mathbf{i} + \sqrt{3}) \mathbf{g}1^{16} \sqrt{-\mathbf{g}1^{48}} - 73 \mathbf{i} (-\mathbf{i} + \sqrt{3}) \mathbf{g}1^{32} \\
& \quad \left. \left( -18 \sqrt{3} (-\mathbf{g}1)^{41/2} \sqrt{-\mathbf{g}1^3} \sqrt{\mathbf{g}1^4} + 35 \sqrt{-\mathbf{g}1^{48}} \right)^{1/3} + 88 (3 \mathbf{i} + \sqrt{3}) (-\mathbf{g}1)^{9/2} \right. \\
& \quad \left. \sqrt{-\mathbf{g}1^3} \sqrt{\mathbf{g}1^4} \sqrt{-\mathbf{g}1^{48}} \left( -18 \sqrt{3} (-\mathbf{g}1)^{41/2} \sqrt{-\mathbf{g}1^3} \sqrt{\mathbf{g}1^4} + 35 \sqrt{-\mathbf{g}1^{48}} \right)^{1/3} - \right. \\
& \quad \left. 36 \sqrt{3} (-\mathbf{g}1)^{41/2} \sqrt{-\mathbf{g}1^3} \sqrt{\mathbf{g}1^4} \left( -18 \sqrt{3} (-\mathbf{g}1)^{41/2} \sqrt{-\mathbf{g}1^3} \sqrt{\mathbf{g}1^4} + 35 \sqrt{-\mathbf{g}1^{48}} \right)^{2/3} + \right. \\
& \quad \left. 70 \sqrt{-\mathbf{g}1^{48}} \left( -18 \sqrt{3} (-\mathbf{g}1)^{41/2} \sqrt{-\mathbf{g}1^3} \sqrt{\mathbf{g}1^4} + 35 \sqrt{-\mathbf{g}1^{48}} \right)^{2/3} \right) \text{MP}^2 \Bigg) \mathbf{f}^2 \Bigg) / \\
& \left( 18 \left( \sqrt{-\mathbf{g}1^3} \left( -18 \sqrt{3} (-\mathbf{g}1)^{41/2} \sqrt{-\mathbf{g}1^3} \sqrt{\mathbf{g}1^4} + 35 \sqrt{-\mathbf{g}1^{48}} \right)^{5/3} \right) \right) + \\
& \left( \mathbf{e}^{3/2} (-\mathbf{g}1)^{141/2} \left( 10\,457\,821\,477 \mathbf{i} (\mathbf{i} + \sqrt{3}) \mathbf{g}1^{44} + 6\,307\,878\,046 (-3 \mathbf{i} + \sqrt{3}) (-\mathbf{g}1)^{33/2} \right. \right. \\
& \quad \left. \sqrt{-\mathbf{g}1^3} \sqrt{\mathbf{g}1^4} \sqrt{-\mathbf{g}1^{48}} + 2\,128\,213\,604 (3 \mathbf{i} + \sqrt{3}) (-\mathbf{g}1)^{65/2} \sqrt{-\mathbf{g}1^3} \sqrt{\mathbf{g}1^4} \right. \\
& \quad \left. \left( -18 \sqrt{3} (-\mathbf{g}1)^{41/2} \sqrt{-\mathbf{g}1^3} \sqrt{\mathbf{g}1^4} + 35 \sqrt{-\mathbf{g}1^{48}} \right)^{1/3} - 2\,001\,760\,259 \mathbf{i} (-\mathbf{i} + \sqrt{3}) \right. \\
& \quad \left. \mathbf{g}1^{12} \sqrt{-\mathbf{g}1^{48}} \left( -18 \sqrt{3} (-\mathbf{g}1)^{41/2} \sqrt{-\mathbf{g}1^3} \sqrt{\mathbf{g}1^4} + 35 \sqrt{-\mathbf{g}1^{48}} \right)^{1/3} + 1\,306\,263\,898 \right. \\
& \quad \left. \mathbf{g}1^{28} \left( -18 \sqrt{3} (-\mathbf{g}1)^{41/2} \sqrt{-\mathbf{g}1^3} \sqrt{\mathbf{g}1^4} + 35 \sqrt{-\mathbf{g}1^{48}} \right)^{2/3} - 177\,241\,680 \sqrt{3} \sqrt{-\mathbf{g}1} \right. \\
& \quad \left. \left. \sqrt{-\mathbf{g}1^3} \sqrt{\mathbf{g}1^4} \sqrt{-\mathbf{g}1^{48}} \left( -18 \sqrt{3} (-\mathbf{g}1)^{41/2} \sqrt{-\mathbf{g}1^3} \sqrt{\mathbf{g}1^4} + 35 \sqrt{-\mathbf{g}1^{48}} \right)^{2/3} \right) \text{MP}^2 \mathbf{f}^4 \right) / \\
& \left( 10\,368 \sqrt{5} \sqrt{-\mathbf{g}1^3} \left( -18 \sqrt{3} (-\mathbf{g}1)^{41/2} \sqrt{-\mathbf{g}1^3} \sqrt{\mathbf{g}1^4} + 35 \sqrt{-\mathbf{g}1^{48}} \right)^{14/3} \right) + \\
& \mathbf{o}[\mathbf{f}]^6, 1\}, \\
& \left\{ \left( \mathbf{e}^{3/2} \left( 13 (1 - \mathbf{i} \sqrt{3}) \mathbf{g}1^{16} + 2 \sqrt{3} (-\mathbf{g}1)^{9/2} \sqrt{-\mathbf{g}1^3} \sqrt{\mathbf{g}1^4} \right. \right. \right. \\
& \quad \left. \left( -18 \sqrt{3} (-\mathbf{g}1)^{41/2} \sqrt{-\mathbf{g}1^3} \sqrt{\mathbf{g}1^4} + 35 \sqrt{-\mathbf{g}1^{48}} \right)^{1/3} + \right. \\
& \quad \left. (1 + \mathbf{i} \sqrt{3}) \left( -18 \sqrt{3} (-\mathbf{g}1)^{41/2} \sqrt{-\mathbf{g}1^3} \sqrt{\mathbf{g}1^4} + 35 \sqrt{-\mathbf{g}1^{48}} \right)^{2/3} \right)^2 \text{MP}^2 \Bigg) / \\
& \left. \left( 32 \sqrt{5} (-\mathbf{g}1)^{27/2} \sqrt{-\mathbf{g}1^3} \left( -18 \sqrt{3} (-\mathbf{g}1)^{41/2} \sqrt{-\mathbf{g}1^3} \sqrt{\mathbf{g}1^4} + 35 \sqrt{-\mathbf{g}1^{48}} \right)^{2/3} \right) \right) -
\end{aligned}$$



$$\left( \left( \sqrt{5} \, e^{3/2} (-g_1)^{5/2} \left( 58 (3i + \sqrt{3}) (-g_1)^{73/2} \sqrt{-g_1^3} \sqrt{g_1^4} - \right. \right. \right.$$
$$601 i (-i + \sqrt{3}) g_1^{16} \sqrt{-g_1^{48}} + 73 i (i + \sqrt{3}) g_1^{32}$$
$$\left. \left( -18 \sqrt{3} (-g_1)^{41/2} \sqrt{-g_1^3} \sqrt{g_1^4} + 35 \sqrt{-g_1^{48}} \right)^{1/3} + 88 (-3i + \sqrt{3}) (-g_1)^{9/2} \right.$$
$$\sqrt{-g_1^3} \sqrt{g_1^4} \sqrt{-g_1^{48}} \left( -18 \sqrt{3} (-g_1)^{41/2} \sqrt{-g_1^3} \sqrt{g_1^4} + 35 \sqrt{-g_1^{48}} \right)^{1/3} -$$
$$36 \sqrt{3} (-g_1)^{41/2} \sqrt{-g_1^3} \sqrt{g_1^4} \left( -18 \sqrt{3} (-g_1)^{41/2} \sqrt{-g_1^3} \sqrt{g_1^4} + 35 \sqrt{-g_1^{48}} \right)^{2/3} +$$
$$70 \sqrt{-g_1^{48}} \left( -18 \sqrt{3} (-g_1)^{41/2} \sqrt{-g_1^3} \sqrt{g_1^4} + 35 \sqrt{-g_1^{48}} \right)^{2/3} \Big) \text{MP}^2 \Big) f^2 \Big) /$$
$$\left( 18 \left( \sqrt{-g_1^3} \left( -18 \sqrt{3} (-g_1)^{41/2} \sqrt{-g_1^3} \sqrt{g_1^4} + 35 \sqrt{-g_1^{48}} \right)^{5/3} \right) \right) +$$
$$\left( e^{3/2} (-g_1)^{141/2} \left( -10457821477 i (-i + \sqrt{3}) g_1^{44} + 6307878046 (3i + \sqrt{3}) (-g_1)^{33/2} \right. \right.$$
$$\sqrt{-g_1^3} \sqrt{g_1^4} \sqrt{-g_1^{48}} + 2128213604 (-3i + \sqrt{3}) (-g_1)^{65/2} \sqrt{-g_1^3} \sqrt{g_1^4}$$
$$\left. \left( -18 \sqrt{3} (-g_1)^{41/2} \sqrt{-g_1^3} \sqrt{g_1^4} + 35 \sqrt{-g_1^{48}} \right)^{1/3} + 2001760259 i (i + \sqrt{3}) g_1^{12} \right.$$
$$\sqrt{-g_1^{48}} \left( -18 \sqrt{3} (-g_1)^{41/2} \sqrt{-g_1^3} \sqrt{g_1^4} + 35 \sqrt{-g_1^{48}} \right)^{1/3} + 1306263898 g_1^{28}$$
$$\left. \left( -18 \sqrt{3} (-g_1)^{41/2} \sqrt{-g_1^3} \sqrt{g_1^4} + 35 \sqrt{-g_1^{48}} \right)^{2/3} - 177241680 \sqrt{3} \sqrt{-g_1} \sqrt{-g_1^3} \right.$$
$$\sqrt{g_1^4} \sqrt{-g_1^{48}} \left( -18 \sqrt{3} (-g_1)^{41/2} \sqrt{-g_1^3} \sqrt{g_1^4} + 35 \sqrt{-g_1^{48}} \right)^{2/3} \Big) \text{MP}^2 f^4 \Big) /$$
$$\left( 10368 \sqrt{5} \sqrt{-g_1^3} \left( -18 \sqrt{3} (-g_1)^{41/2} \sqrt{-g_1^3} \sqrt{g_1^4} + 35 \sqrt{-g_1^{48}} \right)^{14/3} \right) +$$
$$\left. \left. \left. 0[f]^6, 1 \right\} \right\} \right\}$$

Next we simplify and find that the result is a linear function in  $g_1$  and a series in  $f$ :

```
In[107]:= TimeUsed[]
```

Out[107]= 281.811

In[108]:= **simpscalarmassessquared = FullSimplify[scalarmassesfromf3, g1 < 0];**  
**simpscalarmassessquared**

$$\begin{aligned} \text{Out[108]} = & \left\{ \{0, 15\}, \left\{ -\frac{15}{8} \left( \sqrt{5} e^{3/2} g1 MP^2 \right) + \frac{1}{4} \sqrt{5} e^{3/2} g1 MP^2 f^2 + \frac{53 e^{3/2} g1 MP^2 f^4}{576 \sqrt{5}} + O[f]^6, 8 \right\}, \right. \\ & \left\{ -\frac{5}{24} \left( \sqrt{5} e^{3/2} g1 MP^2 \right) - \frac{5}{108} \left( \sqrt{5} e^{3/2} g1 MP^2 \right) f^2 - \frac{245 \left( \sqrt{5} e^{3/2} g1 MP^2 \right) f^4}{15552} + O[f]^6, 6 \right\}, \\ & \left\{ -\frac{15}{8} \left( \sqrt{5} e^{3/2} g1 MP^2 \right) + \frac{1}{3} \sqrt{5} e^{3/2} g1 MP^2 f^2 + \frac{43 \sqrt{5} e^{3/2} g1 MP^2 f^4}{1728} + O[f]^6, 2 \right\}, \\ & \left\{ -\frac{3 \left( e^{3/2} g1 MP^2 \right)}{2 \sqrt{5}} - \frac{\left( e^{3/2} g1 MP^2 \right) f^4}{48 \sqrt{5}} + O[f]^6, 1 \right\}, \\ & \left\{ -\frac{15}{8} \left( \sqrt{5} e^{3/2} g1 MP^2 \right) + \frac{1}{3} \sqrt{5} e^{3/2} g1 MP^2 f^2 + \frac{23 e^{3/2} g1 MP^2 f^4}{192 \sqrt{5}} + O[f]^6, 1 \right\}, \\ & \left. \left\{ -\frac{\left( e^{3/2} g1 MP^2 \right) f^4}{54 \sqrt{5}} + O[f]^6, 1 \right\} \right\} \end{aligned}$$

In[109]:= **Normal[simpscalarmassessquared]**

$$\begin{aligned} \text{Out[109]} = & \left\{ \{0, 15\}, \left\{ -\frac{15}{8} \sqrt{5} e^{3/2} g1 MP^2 + \frac{1}{4} \sqrt{5} e^{3/2} f^2 g1 MP^2 + \frac{53 e^{3/2} f^4 g1 MP^2}{576 \sqrt{5}}, 8 \right\}, \right. \\ & \left\{ -\frac{5}{24} \sqrt{5} e^{3/2} g1 MP^2 - \frac{5}{108} \sqrt{5} e^{3/2} f^2 g1 MP^2 - \frac{245 \sqrt{5} e^{3/2} f^4 g1 MP^2}{15552}, 6 \right\}, \\ & \left\{ -\frac{15}{8} \sqrt{5} e^{3/2} g1 MP^2 + \frac{1}{3} \sqrt{5} e^{3/2} f^2 g1 MP^2 + \frac{43 \sqrt{5} e^{3/2} f^4 g1 MP^2}{1728}, 2 \right\}, \\ & \left\{ -\frac{3 e^{3/2} g1 MP^2}{2 \sqrt{5}} - \frac{e^{3/2} f^4 g1 MP^2}{48 \sqrt{5}}, 1 \right\}, \\ & \left\{ -\frac{15}{8} \sqrt{5} e^{3/2} g1 MP^2 + \frac{1}{3} \sqrt{5} e^{3/2} f^2 g1 MP^2 + \frac{23 e^{3/2} f^4 g1 MP^2}{192 \sqrt{5}}, 1 \right\}, \left. \left\{ -\frac{e^{3/2} f^4 g1 MP^2}{54 \sqrt{5}}, 1 \right\} \right\} \end{aligned}$$

Here it is simplest to just remove the higher terms in  $f$  by hand to get the first approximation to the eigenvalues:

In[110]:= **chopoffbyhandsimpscalarmassessquared :=**

$$\begin{aligned} & \left\{ \{0, 15\}, \left\{ -\frac{15}{8} \sqrt{5} e^{3/2} g1 MP^2, 8 \right\}, \left\{ -\frac{5}{24} \sqrt{5} e^{3/2} g1 MP^2, 6 \right\}, \right. \\ & \left. \left\{ -\frac{15}{8} \sqrt{5} e^{3/2} g1 MP^2, 2 \right\}, \left\{ -\frac{3 e^{3/2} g1 MP^2}{2 \sqrt{5}}, 1 \right\}, \right. \\ & \left. \left\{ -\frac{15}{8} \sqrt{5} e^{3/2} g1 MP^2, 1 \right\}, \left\{ -\frac{e^{3/2} f^4 g1 MP^2}{54 \sqrt{5}}, 1 \right\} \right\} /. e^{3/2} g1 MP^2 \rightarrow -MSP^2 \end{aligned}$$

In[111]:= **chopoffbyhandsimpscalarmassessquared**

$$\begin{aligned} \text{Out[111]} = & \left\{ \{0, 15\}, \left\{ \frac{15 \sqrt{5} MSP^2}{8}, 8 \right\}, \left\{ \frac{5 \sqrt{5} MSP^2}{24}, 6 \right\}, \right. \\ & \left. \left\{ \frac{15 \sqrt{5} MSP^2}{8}, 2 \right\}, \left\{ \frac{3 MSP^2}{2 \sqrt{5}}, 1 \right\}, \left\{ \frac{15 \sqrt{5} MSP^2}{8}, 1 \right\}, \left\{ \frac{f^4 MSP^2}{54 \sqrt{5}}, 1 \right\} \right\} \end{aligned}$$

$$\begin{aligned} \text{In[112]} = & \text{Transpose} \left[ \left\{ \{0, 15\}, \left\{ \frac{15 \sqrt{5} MSP^2}{8}, 8 \right\}, \left\{ \frac{5 \sqrt{5} MSP^2}{24}, 6 \right\}, \right. \right. \\ & \left. \left. \left\{ \frac{15 \sqrt{5} MSP^2}{8}, 2 \right\}, \left\{ \frac{3 MSP^2}{2 \sqrt{5}}, 1 \right\}, \left\{ \frac{15 \sqrt{5} MSP^2}{8}, 1 \right\}, \left\{ \frac{f^4 MSP^2}{54 \sqrt{5}}, 1 \right\} \right\} \right] \end{aligned}$$

$$\begin{aligned} \text{Out[112]} = & \left\{ \left\{ 0, \frac{15 \sqrt{5} MSP^2}{8}, \frac{5 \sqrt{5} MSP^2}{24}, \frac{15 \sqrt{5} MSP^2}{8}, \frac{3 MSP^2}{2 \sqrt{5}}, \frac{15 \sqrt{5} MSP^2}{8}, \frac{f^4 MSP^2}{54 \sqrt{5}} \right\}, \right. \\ & \left. \{15, 8, 6, 2, 1, 1, 1\} \right\} \end{aligned}$$

Now we see that there is one non-zero eigenvalue (the last singlet below) that is much much smaller than the others, because it has a factor of  $f^4$  that they do not have: this is the see saw here, which allows us to get a huge hierarchy between the Higgs and the other scalar masses:

```
In[113]:= truescalarmassssquared := Transpose[chopoffbyhandsimpscalarmassessquared];
truescalarmassssquared
```

```
Out[113]= {{0,  $\frac{15 \sqrt{5} \text{MSP}^2}{8}$ ,  $\frac{5 \sqrt{5} \text{MSP}^2}{24}$ ,  $\frac{15 \sqrt{5} \text{MSP}^2}{8}$ ,  $\frac{3 \text{MSP}^2}{2 \sqrt{5}}$ ,  $\frac{15 \sqrt{5} \text{MSP}^2}{8}$ ,  $\frac{f^4 \text{MSP}^2}{54 \sqrt{5}}$ },
{15, 8, 6, 2, 1, 1, 1}}
```

```
In[114]:= TeXForm[truescalarmassssquared /. MSP → MSP]
```

```
Out[114]//TeXForm=
\left(
\begin{array}{ccccccc}
0 & \&\frac{15}{8} \sqrt{5} M_{\text{SP}}^2 & \&\frac{5}{24} \sqrt{5} M_{\text{SP}}^2 & \&\frac{3}{2 \sqrt{5}} M_{\text{SP}}^2 & \&\frac{15 \sqrt{5}}{8} M_{\text{SP}}^2 & \&\frac{f^4}{54 \sqrt{5}} M_{\text{SP}}^2 \\
15 & 8 & 6 & 2 & 1 & 1 & 1
\end{array}
\right)
```

## The Gravitino Mass and other parameters and results in TeXForm for the paper:

```
In[115]:= (* values of parameters *)
```

```
In[116]:= truevecmasses = Normal[vecmasseswithr /. rexpandedinf[[3]]]; truevecmasses
```

```
Out[116]= {{0, 9}, {40 MP^2 g_5^2 -  $\frac{16}{3} f^2 \text{MP}^2 g_5^2$ , 6},
{ $\frac{8}{5} f^2 \text{MP}^2 g_5^2$ , 1}, {f^2 MP^2 g_5^2, 2}, {40 MP^2 g_5^2 - 7 f^2 MP^2 g_5^2, 6}}
```

```
In[117]:= Transpose[truevecmasses /. MP → MP]
```

```
Out[117]= {{0, 40 g_5^2 M_P^2 -  $\frac{16}{3} f^2 g_5^2 M_P^2$ ,  $\frac{8}{5} f^2 g_5^2 M_P^2$ , f^2 g_5^2 M_P^2, 40 g_5^2 M_P^2 - 7 f^2 g_5^2 M_P^2}, {9, 6, 1, 2, 6}}
```

Again it is simplest to just remove the higher terms in  $f$  by hand to get the first approximation to the eigenvalues:

In[118]:= **handchoptransposetruevecmasses :=**

$$\left\{ \left\{ 0, 40 g_5^2 M_P^2, \frac{8}{5} f^2 g_5^2 M_P^2, f^2 g_5^2 M_P^2, 40 g_5^2 M_P^2 \right\}, \{9, 6, 1, 2, 6\} \right\}$$

In[119]:= **TeXForm[handchoptransposetruevecmasses /. MP → M<sub>P</sub>]**

Out[119]//TeXForm=

```
\left(
\begin{array}{ccccc}
0 & 40 g_5^2 M_P^2 & \frac{8}{5} f^2 g_5^2 M_P^2 & f^2 g_5^2 M_P^2 & 40 g_5^2 M_P^2 \\
9 & 6 & 1 & 2 & 6
\end{array}
\right)
```

In[120]:= **values := {MP → 2.4 × 10<sup>18</sup>, MW → 80.385, MH → 125, M<sub>P</sub> → MP}**

In[121]:= **valueforf := Solve[truevecmasses[[4, 1]] == MW<sup>2</sup>, f] /. values; valueforf**

Out[121]=  $\left\{ \left\{ f \rightarrow -\frac{3.34938 \times 10^{-17}}{g_5} \right\}, \left\{ f \rightarrow \frac{3.34938 \times 10^{-17}}{g_5} \right\} \right\}$

In[122]:= **TeXForm[Flatten[valueforf][[2]]]**

Out[122]//TeXForm=

```
f\to \frac{\text{3.349375}\grave{\text{ }}*\text{\{}^{\wedge}\text{\{-17\}}\}}{g_5}
```

In[123]:= **valueofg1 =**

$$\mathbf{N}\left[\text{Solve}\left[\text{truescalarmassssquared}[[1, 7]] /. \text{MSP} \rightarrow \text{Sqrt}\left[-e^{3/2} g_1 M_P^2\right] == \text{MH}^2, g_1\right] /. \text{valueforf}[[2]] /. \text{values}\right]; \text{valueofg1}$$

Out[123]=  $\left\{ \left\{ g_1 \rightarrow -5.80737 \times 10^{34} g_5^4 \right\} \right\}$

In[124]:= **TeXForm[Flatten[valueofg1][[1]]]**

Out[124]//TeXForm=

```
\text{g1}\to -5.80737\times 10^{\{34\}} g_5^4
```

In[125]:= **Sqrt[-E<sup>3/2</sup> g<sub>1</sub> M<sub>P</sub><sup>2</sup>] /. MP → M<sub>P</sub>**

Out[125]=  $e^{3/4} \sqrt{-g_1 M_P^2}$

In[126]:= **TeXForm[Sqrt[-E<sup>3/2</sup> g<sub>1</sub> M<sub>P</sub><sup>2</sup>] /. MP → M<sub>P</sub>]**

Out[126]//TeXForm=

```
e^{\{3/4\}} \sqrt{-\text{g1} M_P^2}
```

In[127]:= **msuperplanck := Simplify[**

$$\text{Sqrt}\left[-E^{3/2} g_1 M_P^2 /. \text{valueofg1} /. \text{values} /. \text{valueforf}[[2]]\right], g_5 > 0]; \text{msuperplanck}$$

Out[127]=  $\{1.2244 \times 10^{36} g_5^2\}$

In[128]:= **TeXForm[msuperplanck]**

Out[128]//TeXForm=

```
\left\{\text{1.2244}\times 10^{\{36\}} g_5^2\right\}
```

```

In[129]:= gravitinomassssquared1 :=
  FullSimplify[(1/(MP^4)) prefactorforscalarmassssquared Abs[WbShifted^2] /.
    replaceAllFieldsWithZero]

In[130]:= gravitinomassssquared1

Out[130]= 
$$\left( e^{3 - \text{Re}\left[\frac{MK1^2 + MK2^2 + MK9^2}{b MP^2}\right]} \text{Abs}\left[\left(4 \sqrt{15} g_1 MK2 (9 MK1^2 + MK2^2) + 3 g_2 (5 MK1 - \sqrt{15} MK2) MK9^2\right) MP^3\right] \right) / (60 \sqrt{2} MP^4)$$


In[131]:= gravitinomassssquared2 :=
  gravitinomassssquared1 /. rnewsol15 /. g2 → r g1 /. rbigtof[[3]] /. f → 0 /. values

In[132]:= gravitinomassssquared3 := Simplify[gravitinomassssquared2 /. valueofg1, g5 > 0]

In[133]:= gravitinomassssquared3

Out[133]=  $\left\{1.80282 \times 10^{73} e^{-6 \text{Re}\left[\frac{1}{b}\right]} g_5^4\right\}$ 

In[134]:= gravitinomass := Simplify[Sqrt[gravitinomassssquared3 /. b → 4], g5 > 0]

In[135]:= gravitinomass

Out[135]=  $\{2.00565 \times 10^{36} g_5^2\}$ 

In[136]:= TeXForm[gravitinomass]

Out[136]/TeXForm=
  \left\{2.00565\times 10^{36} g_5^2\right\}

In[137]:= geVtograms := 1.78 × 10-24

In[138]:= geVtograms

Out[138]= 1.78 × 10-24

In[139]:= gravitinomass geVtograms

Out[139]=  $\{3.57006 \times 10^{12} g_5^2\}$ 

In[140]:= msuperplanck geVtograms

Out[140]=  $\{2.17942 \times 10^{12} g_5^2\}$ 

In[141]:= TeXForm[msuperplanck geVtograms]

Out[141]/TeXForm=
  \left\{2.17942\times 10^{12} g_5^2\right\}

In[142]:= MW / MP /. values

Out[142]= 3.34938 × 10-17

In[143]:= MH / MP /. values

Out[143]= 5.20833 × 10-17

```

```
In[144]:= N[Transpose[Simplify[Thread[Sqrt[truescalarmassssquared]]]]][[1]]
```

```
Out[144]= {0., 2.04759  $\sqrt{\text{MSP}^2}$ , 0.68253  $\sqrt{\text{MSP}^2}$ , 2.04759  $\sqrt{\text{MSP}^2}$ ,  
0.819036  $\sqrt{\text{MSP}^2}$ , 2.04759  $\sqrt{\text{MSP}^2}$ , 0.091004  $\sqrt{f^4 \text{MSP}^2}$ }
```

```
In[145]:= TeXForm[N[Transpose[Simplify[Thread[Sqrt[truescalarmassssquared]]]]][[1]]]
```

```
Out[145]/TeXForm=  
\left\{0., 2.04759 \sqrt{\text{MSP}^2}, 0.68253 \sqrt{\text{MSP}^2}, 2.04759  
 \sqrt{\text{MSP}^2}, 0.819036 \sqrt{\text{MSP}^2}, 2.04759 \sqrt{\text{MSP}^2}, 0.0  
 \sqrt{f^4 \text{MSP}^2}\right\}
```

```
In[146]:= gravitinomass / msuperplanck
```

```
Out[146]= {1.63807}
```

```
In[147]:= TimeUsed[]
```

```
Out[147]= 326.155
```

```
In[148]:= UnitConvert[326.155 s, MixedRadix["Minutes", "Seconds"]]
```

```
Out[148]= 5 min 26.155 s
```
